# Supplementary material for: Event-Keyed Summarization
Source: arXiv:2402.06973 source file (2024-02-10)
Supplement: Supplementary file 1 [file additional_results.tex]

% \begin{table}[]
%     \centering
%     \adjustbox{max width = \columnwidth}{
%     \begin{tabular}{ll|cccccc}
%     \toprule
%     & & Gold$\rightarrow$Gen & Gold$\leftarrow$Gen & Average & Doc$\rightarrow$Gen & Doc$\rightarrow$Gen & Doc$\rightarrow$Gold\\
%     \midrule
%     & temp + doc & 39.9 & 30.6 & 35.2 & 37.4 & 37.4 & 41.2\\
%     $\textsc{BART}$ & temp only & 15.4 & 8.8 & 12.1 & 12.2 & 12.2 & 41.2\\
%     & doc only & 18.3 & 11.8 & 15.1 & 41.0 & 41.0 & 41.2\\
%     \midrule
%     & temp + doc & 36.8 & 28.5 & 32.6 & 40.6 & 40.6 & 41.2\\
%     $\textsc{PEGASUS}$ & temp only & 30.6 & 7.9 & 19.3 & 19.8 & 19.8 & 41.2\\
%     & doc only & 18.8 & 13.0 & 15.9 & 42.2 & 42.2 & 41.2\\
%     \midrule
%     & temp + doc & 43.1 & 30.5 & 36.8 & 40.6 & 40.6 & 41.2\\
%     $\textsc{T5}$ & temp only & 27.4 & 7.6 & 17.5 & 16.5 & 16.5 & 41.2\\
%     & doc only & 18.2 & 12.5 & 15.3 & 42.4 & 42.4 & 41.2\\
%     \midrule
%     & temp + doc & \textbf{-} & \textbf{-} & \textbf{-} & \textbf{-} & -\\ % 770M 
%     $\textsc{Llama7B}$ & temp only & - & - & - & - & -\\
%     & doc only & - & - & - & - & -\\
%     \midrule
%     & temp + doc & 30.6 & 43.0 & 36.8 & 40.8 & 40.8 & 41.2\\
%     $\textsc{ChatGPT}$ & temp only & - & - & - & - & -\\
%     & doc only & - & - & - & - & -\\
%     \midrule
%     & temp + doc & 45.0 & 40.3 & 42.7 & 38.8 & 38.8 & 41.2\\
%     $\textsc{GPT4}$ & temp only & - & - & - & - & -\\
%     & doc only & - & - & - & - & -\\
%     \bottomrule
%     \end{tabular}
%     }
%     \caption{NLI Evaluation for the models}
%     \label{tab:nli_eval}
% \end{table}

% \begin{table}[h]
%     \centering
%     \begin{tabular}{l|ccc}
%     \toprule
%          & \textbf{P} & \textbf{R} & $\textbf{F}_1$ \\
%     \midrule
%         BART & 78.6 & 66.0 & 71.8 \\
%         PEGASUS & 74.0 & 62.3 & 67.6 \\
%         T5 & 80.6 & 63.3 & 70.9 \\
%         ChatGPT & 57.7 & 62.9 & 60.2 \\
%         GPT-4 & 70.2 & 65.2 & 67.6 \\
%     \bottomrule
%     \end{tabular}
%     \caption{CEAF-REE scores for temp+doc models, averaged over three runs/prompts}
%     \label{tab:ceaf_ree_scores}
% \end{table}
