# Supplementary material for: Event-Keyed Summarization
Source: arXiv:2402.06973 source file (2024-02-10)
Supplement: Supplementary file 2 [file temp-lit-review.tex]

\subsection{Information Extraction based Summarization}
\paragraph{\cite{s-hussain-etal-2022-event}} some stuff


\paragraph{\cite{}}


\subsection{Controlled Summarization}
\paragraph{\cite{fan-etal-2018-controllable}} Summaries to follow user preferences. 

\paragraph{\cite{he-etal-2022-ctrlsum}} Summaries for user preferences, also event-centric



\subsection{Evaluating Eval Metrics}
\paragraph{\cite{deutsch-etal-2021-statistical}} An evaluation of evaluation metrics shows high uncertainty in the reliability of automatic metrics. 

\paragraph{\cite{fabbri-etal-2021-summeval}}


\paragraph{Looking for a Few Good Metrics: Automatic Summarization Evaluation - How Many Samples Are Enough?} evaluating against multiple references results in higher correlation scores with human judgments. however, a single-reference setting is sufficient for the metric to be effective


\paragraph{\cite{rankel-etal-2013-decade}} variants of the ROUGE metric using TAC datasets.


\paragraph{\cite{graham-2015-evaluating}} different ROUGE metric variants and compared it against the BLEU metric on the DUC datasets.

\paragraph{\cite{maynez-etal-2020-faithfulness}} "However, our analysis does show that pretrained models are better summarizers not only in terms of raw metrics, i.e., ROUGE, but also in generating faithful and factual summaries as evaluated by humans. Furthermore, we show that textual entailment measures better correlate with faithfulness than standard metrics, potentially leading the way to automatic evaluation metrics as well as training and decoding criteria.
